# Supplementary material for: Verifying Text Summaries of Relational Data Sets
Source: arXiv:1804.07686 source file (2018-08-30)
Supplement: Supplementary file 1 [file appendix.tex]

\begin{table}[t]
	\caption{Annotation Type.}
	\scalebox{0.9}{
		\begin{tabular}{cl}
			\toprule
			\textbf{Annotation} & \textbf{Description} \\
			\midrule
			Correct & Claim \& Consistent with the data set\\
			Wrong & Claim \& Inconsistent with the data set\\
			Complex & Claim\\&\& Do not comply with SQL format of FactChecker\\
			Uncertain & Claim \& Underlying SQL query is unknown\\
			Missing Data & Claim \& From some other data set\\
			Not a Claim & Not a claim\\
			\bottomrule
		\end{tabular}
	}
	\label{tab:annotation_types}
\end{table}

\begin{figure*}
\centering
\subfigure[Annotation types.\label{fig:annotationType}]
{
	\includegraphics[width=0.3\textwidth]{plots/annotationTypeRatio.pdf}
}
\subfigure[Claim types.\label{fig:annotationType2}]
{
	\includegraphics[width=0.3\textwidth]{plots/annotationTypeRatio_OfInterest.pdf}
}
\subfigure[Claim types.\label{fig:annotationType3}]
{
	\includegraphics[width=0.3\textwidth]{plots/annotationTypeRatio_Correctness.pdf}
}
\caption{Distribution of statistical claims according to different criteria.\label{fig:annotation}}
\end{figure*}

\begin{figure*}
	\centering
	\subfigure[Usability.\label{fig:userStudyRating_Compare}]
	{
		\includegraphics[width=0.35\textwidth]{plots/userStudyRatingComparison_SQLExperience.pdf}
	}
	\subfigure[Usefulness of each recommendation features.\label{fig:userStudyRating_Feature}]
	{
		\includegraphics[width=0.35\textwidth]{plots/userStudyRatingFeature_SQLExperience.pdf}
	}
	\caption{User rating of the FactChecker compared to an SQL interface.\label{fig:userStudyRating}}
\end{figure*}

\begin{figure}
	\includegraphics[width=0.4\textwidth]{plots/wrongStatistics.pdf}
	\caption{Recall and precision of incorrect claims in three cases: User-operated FactChecker, User-operated SQL interface, and Unsupervised FactChecker. \label{fig:wrongStatistics}}
\end{figure}

\begin{figure*}
	\centering
		\subfigure[Different document sources.\label{fig:topNQueries_Article}]
		{
			\includegraphics[width=0.35\textwidth]{plots/topNQueriesRatio_Article.pdf}
		} 
		\subfigure[Markup by FactChecker.\label{fig:topNQueries_Verified}]
		{
			\includegraphics[width=0.35\textwidth]{plots/topNQueriesRatio_Verified.pdf}
		}
	\caption{Accuracy of top-N mostly likely query recommendations.\label{fig:topNQueries_Remainder}}
\end{figure*}

\begin{figure*}
	\centering
	\subfigure[Top-N Aggregation Function Recommendation.\label{fig:topNAggFunction}]
	{
		\includegraphics[width=0.35\textwidth]{plots/topNAggFunctionRatio.pdf}
	}
	\subfigure[Top-N Aggregated Column Recommendation.\label{fig:topNAggColumn}]
	{
		\includegraphics[width=0.35\textwidth]{plots/topNAggColumnRatio.pdf}
	}
	\caption{Accuracy of top-N mostly likely aggregation function and aggregated column recommendations.\label{fig:topN}}
\end{figure*}

\begin{figure}
	\includegraphics[width=0.4\textwidth]{plots/aggFunctionRatioStacked.pdf}
	\caption{Distribution of SQL queries according to aggregation functions.\label{fig:aggFunction}}
\end{figure}

\begin{figure}
	\includegraphics[width=0.4\textwidth]{plots/userStudyPerMinuteByDifficulty.pdf}
	\caption{Number of correctly verified claims per minute.\label{fig:userStudyPerMinuteByDifficulty}}
\end{figure}

\begin{figure}
	\includegraphics[width=0.4\textwidth]{plots/performanceStackoverflow.pdf}
	\caption{Performance improvement by applying different strategies for SQL query execution - Stackoverflow documents (in log scale).\label{fig:performanceStackoverflow}}
\end{figure}

\begin{figure}
	\includegraphics[width=0.4\textwidth]{plots/userStudyFeature.pdf}
	\caption{Percentage of usage of each feature for selecting the matching SQL query in the FactChecker.\label{fig:userStudyFeature}}
\end{figure}

%\begin{figure*}
%	\centering
%	\subfigure[Number of aggregation functions (1 \textasciitilde{} 5).\label{fig:timeAccuracy2_AggFunc}]
%	{
%		\includegraphics[width=0.235\textwidth]{plots/timeAccuracy_AggFunction_v2.pdf}
%	} 
%	\subfigure[Number of aggregated columns (1 \textasciitilde{} 20).\label{fig:timeAccuracy2_AggColumn}]
%	{
%		\includegraphics[width=0.235\textwidth]{plots/timeAccuracy_AggColumn_v2.pdf}
%	}
%	\subfigure[Number of restricted columns (1 \textasciitilde{} 10).\label{fig:timeAccuracy2_RestrictColumn}]
%	{
%		\includegraphics[width=0.235\textwidth]{plots/timeAccuracy_RestrictColumn_v2.pdf}
%	}
%	\subfigure[Number of EM iterations (1 \textasciitilde{} 10).\label{fig:timeAccuracy2_MaxIterationEM}]
%	{
%		\includegraphics[width=0.235\textwidth]{plots/timeAccuracy_MaxIterationEM_v2.pdf}
%	}
%	\caption{Accuracy of FactChecker with varying amount of processing overhead. As the FactChecker utilize more processing power, also the accuracy generally increases except for the number of restricted columns.\label{fig:timeAccuracy2}}
%\end{figure*}
