# Supplementary material for: Verifying Text Summaries of Relational Data Sets
Source: arXiv:1804.07686 source file (2018-08-30)
Supplement: Supplementary file 2 [file appendix2.tex]

\section{Additional Baselines}
We compare FactChecker with the following baselines from various fields including automated fact-checking, natural language querying, and argument mining. ClaimBuster~\cite{HassanA17, HassanZ17} is an automated fact-checking system which allows users to verify natural language texts against other natural language claims validated by human fact checkers. NaLIR~\cite{Li2014} is a natural language querying interface system which translates natural language sentences to SQL queries for relational databases. MARGOT~\cite{LippiT16} is a online argument mining system which identifies potential claims and their supporting evidence from a natural language text. The results demonstrate that these systems address seemingly similar but largely different problems targeting varying application scenarios.

\begin{comment}
\begin{figure}
	\begin{tikzpicture}[font=\small]
	\pie[radius=1, text=legend, color={blue!50, blue!10}]{97/Unsupported, 3/Incorrect Translation}
	\end{tikzpicture}
	\caption{Breakdown of claims by result of NaLIR.\label{nalirBreakdownFig}}
\end{figure}
\end{comment}

\textbf{Experimental Setting.}
ClaimBuster have three types of fact-checking methods which mainly differ in the repository the system utilizes to verify claims: Fact Matcher (ClaimBuster-FM), Knowledge Bases (ClaimBuster-KB), and Search Engine. Given a claim, ClaimBuster-FM searches a repository of fact-checked statements and outputs the most similar statements, each with a similarity rating and a truth rating. We use two different ways of integrating the result of ClaimBuster-FM (i.e., statements) in verifying a claim as either correct or wrong. First approach is to decide based on the truth rating of a statement with the highest similarity score. In a second approach, we group statements according to their truth rating and calculate the sum of similarity scores per truth rating. Then, the truth rating with the highest weighted sum is used to verify a claim. ClaimBuster-KB fact-checks a claim based on the results from Google Answer Boxes and Wolfram Alpha API. To be more precise, ClaimBuster-KB converts a claim into one or multiple questions using a question generation tool~\cite{HeilmanS09, HeilmanS10} and outputs the answers from knowledge base APIs by querying the generated questions. Since the answers do not give similarity ratings, we classify a claim as either correct or wrong based on the most frequent truth rating. We exclude the search engine version of ClaimBuster because the web search results do not include truth ratings.

NaLIR targets natural language query answering where the purpose is to translate a natural language query to an SQL query for relational database. However, NaLIR only supports the translation of a restricted set of natural language sentences which comply with system-specific requirements. To mitigate this issue, we try as inputs not only the original sentence but also the sentences created by the question generating tool used in ClaimBuster-KB. We calculate the recall, precision and F1 score by verifying whether the SQL query generated by NaLIR correctly matches the meaning of its natural language form.

Note that the problem setting of FactChecker is different from that of NaLIR. Our system focuses on a different scenario where multiple relevant claims along with the whole text document is given as input. Furthermore, each claim (i.e., natural language description of a SQL query result) is accompanied with its claimed value, which calls for a novel solution exploiting these properties. 

The main goal of MARGOT is, given a text document, to identify parts of the document that form argument structures (i.e., claims and evidence). Unlike the FactChecker, MARGOT does not provide any means of fact-checking claims against external sources including their associated data sets. Since MARGOT does not verify the correctness of a claim, it is difficult to directly compute the recall, precision, and F1 score of erroneous claims. Instead, we calculate an upper bound of these values by considering a system that extends MARGOT to support fact-checking. First, we assume that there is a fact-checking system based on MARGOT. Then in prior to fact-checking, it is necessary for the system to correctly identify the claims that should be verified. In this context, the number of erroneous claims that were spotted by MARGOT gives us an upper bound on the performance of the system.

\begin{table}
	\caption{Comparison of FactChecker with other baselines.\label{baselineComparisonTable}}
	\begin{small}
		\begin{tabular}{lrrr}
			\toprule[1pt]
			\textbf{Tool} & \textbf{Recall} & \textbf{Precision} & \textbf{F1 Score} \\
			\midrule[1pt]
			FactChecker Automatic & 50\% & 40\% & 44\% \\
			\midrule
			ClaimBuster-FM (Highest score) & 21\% & 4\% & 7\% \\
			\midrule
			ClaimBuster-FM (Weighted sum) & 14\% & 4\% & 6\% \\
			\midrule
			ClaimBuster-KB & 0\% & 0\% & 0\% \\
			\midrule
			NaLIR & 0\% & 0\% & 0\% \\
			\midrule
			MARGOT & 0\% & 0\% & 0\% \\
			\bottomrule[1pt]
		\end{tabular}
	\end{small}
\end{table}

\begin{table}
	\caption{Comparison on Wikipedia articles.\label{wikipediaComparisonTable}}
	\begin{small}
		\begin{tabular}{lrrr}
			\toprule[1pt]
			\textbf{Tool} & \textbf{Recall} & \textbf{Precision} & \textbf{F1 Score} \\
			\midrule[1pt]
			FactChecker Automatic & 17\% & 50\% & 25\% \\
			\midrule
			\makecell[cl]{FactChecker Automatic\\ (Significant Digits)} & 67\% & 80\% & 73\% \\
			\midrule
			ClaimBuster-KB & 0\% & 0\% & 0\% \\
			\bottomrule[1pt]
		\end{tabular}
	\end{small}
\end{table}

\begin{table}
\center
\caption{Test cases.\label{testCasesTable}}
\begin{footnotesize}
	\begin{tabular}{p{8cm}}
		\toprule[1pt]
		\textbf{Title [Source]} \\
		\midrule[1pt]
		\textbf{[538]} \\
		`Straight Outta Compton' Is The Rare Biopic Not About White Dudes \\
		41 Percent Of Fliers Think You're Rude If You Recline Your Seat \\
		A Complete Catalog Of Every Time Someone Cursed Or Bled Out In A Quentin Tarantino Movie \\
		A Statistical Analysis of the Work of Bob Ross \\
		Blatter's Reign At FIFA Hasn't Helped Soccer's Poor \\
		Dear Mona Followup: Where Do People Drink The Most Beer, Wine And Spirits? \\
		Dear Mona, How Many Flight Attendants Are Men? \\
		Dear Mona, Which State Has The Worst Drivers? \\
		Every Guest Jon Stewart Ever Had On `The Daily Show' \\
		Hip-Hop Is Turning On Donald Trump \\
		How Baby Boomers Get High \\
		How Many Americans Are Married To Their Cousins? \\
		How To Break FIFA \\
		Joining The Avengers Is As Deadly As Jumping Off A Four-Story Building \\
		Pols And Polls Say The Same Thing: Jeb Bush Is A Weak Front-Runner \\
		Should Travelers Avoid Flying Airlines That Have Had Crashes in the Past? \\
		Sitting Presidents Give Way More Commencement Speeches Than They Used To \\
		The NFL's Uneven History Of Punishing Domestic Violence \\
		The Rock Isn't Alone: Lots Of People Are Worried About `The Big One' \\
		Where People Go To Check The Weather \\
		Where Police Have Killed Americans In 2015 \\
		\midrule
		\textbf{[NYT]} \\
		A Lot of Places Resemble Ferguson, Statistically \\
		A Mysterious Republican Committee in the Virgin Islands \\
		Charlie Rangel's Charitable Giving Shrinks Along With Fund-Raising Clout \\
		How Eric Cantor's Defeat Could Hurt Republican Fund-Raising \\
		Looking for John McCain? Try a Sunday Morning Show \\
		Maiden Names, on the Rise Again \\
		Race in `Waxman' Primary Involves Donating Dollars \\
		Yea, Oops, Nay: Voting Mistakes in Congress \\
		\midrule
		\textbf{[Vox]} \\
		Here's every type of data exposed in the Ashley Madison hack \\
		Low-income Americans can no longer afford rent, food, and transportation \\
		\midrule
		\textbf{[Stack Overflow]} \\
		2015 Developer Survey \\
		Developer Survey Results 2016 \\
		Developer Survey Results 2017 \\
		\midrule
		\textbf{[Wikipedia]} \\
		County (United States) \\
		Economy of the European Union \\
		List of Manchester United F.C. records and statistics \\
		\bottomrule[1pt]
	\end{tabular}
\end{footnotesize}
\end{table}

\begin{table*}
\center
\caption{Erroneous Claims.\label{erroneousClaimsTable}}
\begin{small}
	\begin{tabular}{p{6cm}p{8cm}r}
		\toprule[1pt]
		\textbf{Erroneous Claim} & \textbf{Author Comment} & \textbf{Correct Value} \\
		\midrule[1pt]
		There were only \textbf{four} previous lifetime bans in my database - three were for repeated substance abuse, one was for gambling.~\cite{53814-2} & Yes -- the data was updated on Sept. 22, and the article was originally published on Aug. 28. There's a note at the end of the article, but you're right the article text should also have been updated. & 6 \\
		\midrule
		There were only four previous lifetime bans in my database - \textbf{three} were for repeated substance abuse, one was for gambling.~\cite{53814-2} & Yes -- the data was updated on Sept. 22, and the article was originally published on Aug. 28. There's a note at the end of the article, but you're right the article text should also have been updated. & 4 \\
		\midrule
		Obama has spoken widely, in \textbf{17} states and D.C., while giving commencement addresses no more than three times in any one state (New York).~\cite{53816-2} & ... the likely explanation is that the data on GitHub does not include speeches Obama gave in 2016. & 16 \\
		\midrule
		Using their campaign fund-raising committees and leadership political action committees separately, the pair have given money to \textbf{64} candidates.~\cite{NYT14-2} & I think you are correct in that it should be 63 candidates in the article, not 64. & 63 \\
		\midrule
		This year, \textbf{56,033} coders in 173 countries answered the call.~\cite{Stackoverflow16}& Our analyst's recollection is that three of the responses were from people who "stumbled" into the survey and had no business taking it, so they were excluded from the data file and the reporting... but meanwhile, the team building the website were writing copy based on the initial count of respondents. & 56,030 \\
		\midrule
		\textbf{13\%} of respondents across the globe tell us they are only self-taught.~\cite{Stackoverflow16} & This was a rounding error/typo on our part -- so yes, you're correct. & 14 \\
		\bottomrule[1pt]
	\end{tabular}
\end{small}
\end{table*}

\begin{table}
\caption{Amazon Mechanical Turk Results.\label{AMTTable}}
\begin{small}
	\begin{tabular}{lrrr}
		\toprule[1pt]
		\textbf{Tool} & \textbf{Recall} & \textbf{Precision} & \textbf{F1 Score} \\
		\midrule[1pt]
		FactChecker & 86\% & 96\% & 91\% \\
		\midrule
		Google Spreadsheet & 42\% & 95\% & 58\% \\
		\bottomrule[1pt]
	\end{tabular}
\end{small}
\end{table}

\begin{table}
\center
\caption{Results of user survey.\label{detailedSurveyTable}}
\begin{small}
	\begin{tabular}{lrrrrr}
		\toprule[1pt]
		\textbf{Criterion} & $\mathbf{SQL++}$ & $\mathbf{SQL+}$ & $\mathbf{SQL\approx FC}$ & $\mathbf{FC+}$ & $\mathbf{FC++}$ \\
		\midrule[1pt]
		Overall & 0 & 0 & 0 & 3 & 5 \\
		\midrule
		Learning & 0 & 0 & 0 & 2 & 6 \\
		\midrule
		Correct Claims & 0 & 0 & 0 & 1 & 7 \\
		\midrule
		Incorrect Claims & 0 & 0 & 1 & 3 & 4 \\
		\bottomrule[1pt]
	\end{tabular}
\end{small}
\end{table}

\textbf{Data set.}
We use the same set of 34 articles and reports as in Section~\ref{experimentsSec} to evaluate the recall, precision, and F1 score on erroneous claims. There are 16 erroneous claims in the text documents where some of the claims appear in the same sentence. Therefore, there are a total of 14 sentences that contain erroneous claims. Since ClaimBuster and NaLIR consider one complete sentence as input, we evaluate these systems on the 14 sentences with erroneous claims. For FactChecker and MARGOT, we compute the result based on 16 erroneous claims.

In addition, we test FactChecker and ClaimBuster-KB on three Wikipedia articles about economy~\cite{wikiEEU}, sports~\cite{wikiLMUFC}, and geography~\cite{wikiCUS}. After the experiment using our original test cases, we noticed that ClaimBuster-KB performs worse than we anticipated despite its ability to access data in knowledge bases. Thus, we decided to prepare additional data sets that we thought would be most favorable to ClaimBuster-KB. Compared to the previous 34 text documents, Wikipedia articles give ClaimBuster-KB much more of an advantage since the claims in these articles are mostly based on popular public data that Google Answer Boxes and Wolfram Alpha API also have access to.

There are 6 erroneous claims out of a total of 24 claims in three Wikipedia articles, surprisingly more than we expected. In terms of sentences, there are a total of 4 sentences with erroneous claims.

\textbf{Results.}
Table~\ref{baselineComparisonTable} demonstrates that our system outperforms other baselines by a large margin in recall, precision and F1 score. The result is primarily due to the difference in the problems that these systems want to solve. The main goal of our system is to fact-check claims about numerical aggregates of the relational data. In contrast, ClaimBuster mainly supports the verification of claims which can be disputed by already fact-checked natural language statements. NaLIR only supports a subset of sentence types which comply with system specifications. Only 3\% of the claims are translated to SQL queries using NaLIR, and even worse, all of the translated SQL queries are incorrect (i.e., not complying with the natural language descriptions of claims). Moreover, ClaimBuster and NaLIR only accepts as input one natural language sentence instead of the whole article, which limits the performance of these systems when a single claim spans over multiple sentences. The objective of MARGOT is to automatically spot arguments from a natural language text and extract the reasoning structure of arguments composed of claims and evidence. Thus, the type of claims that MARGOT focuses on differs from that of FactChecker. Only 1 out of 232 claims from FactChecker's test cases is identified as a claim by MARGOT. Among 16 erroneous claims, none of them is recognized by MARGOT.

Table~\ref{wikipediaComparisonTable} reports recall, precision and F1 score of FactChecker and ClaimBuster-KB on the Wikipedia articles. In Table~\ref{wikipediaComparisonTable}, FactChecker Automatic (Significant Digits) refers to the version of FactChecker where we take into account the significant digits of claimed value in evaluating query results. For instance, a query result like $8.04$, $8.2$, or $8$ is not matched to a claimed value of $8.1$ even though all the numbers round up to $8$. Instead, a query result like $8.1$, $8.13$, or $8.09$ is considered as a match since we consider the significant digits of the claimed value.

Despite choosing carefully the test cases where ClaimBuster-KB could work well, the system still fails to correctly verify erroneous claims in Wikipedia articles. The shortcomings of ClaimBuster-KB include cases where the description of one claim is distributed across multiple sentences or multiple claims are located in the same sentence. Besides these issues, ClaimBuster-KB's approach still suffers from three difficulties: 1) producing the correct question given a claim, which heavily depends on the performance of the question generating tool, 2) giving the correct answer to the question, which depends on the performance of knowledge base APIs, and 3) determining whether answers from knowledge base APIs match the description of the claim. For example, the answer to claim ``In 2015 Ireland had the highest GDP growth of all the states in EU (26.3\%)'' could be found by issuing questions like ``What is the GDP growth of Ireland in 2015'' to Wolfram Alpha API. Nevertheless, the question generating tool used in ClaimBuster-KB fails to create the correct question where the closest attempt is ``What did Ireland have the highest GDP growth of in 2015.''

\begin{figure*}
	\begin{tikzpicture}
	\begin{axis}[ybar=0pt, bar width=2pt, width=14cm, height=4cm, xlabel=Articles, ylabel={Run Time (s)}, ylabel near ticks, xlabel near ticks, ymajorgrids, legend entries={Naive, +Merging, +Caching, +Incremental}, legend pos=outer north east, xtick=\empty, legend style={font=\small}, ymode=log, enlarge x limits=0.05, cycle list name=patternList]
	\addplot table[x expr=\coordindex, y index=1, col sep=comma] {plots/performanceAllArticles.txt};
	\addplot table[x expr=\coordindex, y index=2, col sep=comma] {plots/performanceAllArticles.txt};
	\addplot table[x expr=\coordindex, y index=3, col sep=comma] {plots/performanceAllArticles.txt};
	\addplot table[x expr=\coordindex, y index=5, col sep=comma] {plots/performanceAllArticles.txt};
	\end{axis}
	\end{tikzpicture}
	\caption{Comparison of execution times for different articles and different processing strategies.\label{comparisonByArticleFig}}
\end{figure*}

\begin{figure}
	\begin{tikzpicture}
	\begin{axis}[ybar=0pt, bar width=2pt, width=8.5cm, height=3cm, xlabel=Articles, ylabel={\# Queries}, ylabel near ticks, xlabel near ticks, ymajorgrids, xtick=\empty, legend style={font=\small}, ymode=log]
	\addplot table[x expr=\coordindex, y index=1] {plots/nrPossibleQueriesPGF.txt};
	\end{axis}
	\end{tikzpicture}
	\caption{Number of possible query candidates per data set.\label{nrPossibleQueriesFig}}
\end{figure}

\begin{figure}
	\begin{tikzpicture}
	\begin{axis}[width=6cm, height=3cm, xlabel={$p_T$}, ylabel={}, ylabel near ticks, xlabel near ticks, legend entries={Recall, Precision, F1 Score}, legend pos=outer north east, ymajorgrids, legend style={font=\small}, cycle list name=markerList]
	\addplot table[x index=0, y index=1, col sep=comma] {plots/recallPrecisionTradeOff.txt};
	\addplot table[x index=0, y index=2, col sep=comma] {plots/recallPrecisionTradeOff.txt};
	\addplot table[x index=0, y index=3, col sep=comma] {plots/recallPrecisionTradeOff.txt};
	\end{axis}
	\end{tikzpicture}
	\caption{Effect of parameter $p_T$ on recall and precision.\label{pTFig}}
\end{figure}

\section{More User Study}
\subsection{Amazon Mechanical Turk}
We conducted an additional user study using Amazon Mechanical Turk (AMT), a crowdsourcing platform which allows our system to be tested by anonymous workers. Table~\ref{AMTTable} demonstrates that workers using our system achieved twice the recall of those using Google Spreadsheet.

\textbf{Experimental Setting.}
We generated microtasks where workers were asked to fact-check two specific sentences in an article against its associated dataset using either FactChecker or Google Spreadsheet. Only one of the two sentences contained an erroneous claim, which we used to calculate recall and precision. Since we wanted to make sure workers using Google Spreadsheet could easily verify the claims, we selected simple claims on a small data set (i.e., claims that could be counted by hand). One example is ``\textit{the number of states President Obama have visited to give commencement speeches}'' whose answer is 16. We ensured that any particular worker processes at most one assignment and gathered 50 answers for each tool. The price of a microtask was 50 cents, and we did not set any restrictions on eligible workers. We put the microtasks online for 24 hours starting from 16:48:36 PST on Sunday.

\textbf{Results.}
The results are summarized in Table~\ref{AMTTable}. FactChecker outperforms Google Spreadsheet by double in recall, equals in precision, and an increase from 58\% to 91\% in F1 score. The results are even more impressive given that we did not provide any tutorial or training of our system to workers. Instead, we provided minimum guidelines with few sentences describing our system.

\subsection{User Preferences}
We provide more details on our experimental results with regards to user preferences. Table~\ref{detailedSurveyTable} shows the results of our user survey, following the fact-checking part of the user study, in more detail. We asked users for preferences when comparing SQL to the FactChecker interface. Our scale ranges from a strong preference for SQL (represented a \textbf{SQL++} in Table~\ref{detailedSurveyTable}), over equal preferences ($\mathbf{SQP\approx FC}$), up to a strong preference for the FactChecker (\textbf{FC++}). 

Besides asking for general preferences, we also asked users to compare tools according to specific categories. Namely, we asked about learning overheads, preference for verifying correct claims, and for verifying incorrect claims. 

Users generally prefer the FactChecker. Users perceive the interface as very intuitive and were able to use it with minimal learning overheads. We obtain slightly better results for verifying correct claims than for verifying incorrect claims. This might relate to the recognition accuracy which is indeed higher for correct claims. 

We also collected free form comments from our users. Comments were generally favorable towards our system. A few examples follow. ``\textit{Shortened time considerably. Very Very friendly to non-cs majors. Interface is very simple and easy to follow. I was able to finish all the ones that I used Face Checker before the time ran out so it's awesome. If I had to choose between SQL and Face Checker, I'd choose Fact Checker any day.}`` ``\textit{Really liked that it showed the result of the recommended queries. The suggestions made it very easy to create custom queries.}'' ``\textit{It was very quick and easy to verify correct statistics when it formulated the correct query.}''

\section{Details of Test Cases}
\label{testcasesAppendix}
All test cases used in the paper are summarized in Table~\ref{testCasesTable}. Table~\ref{erroneousClaimsTable} presents a selection of erroneous claims from our test data sets. We added comments that we received by email from the writers of the text documents. Figure~\ref{nrPossibleQueriesFig} shows for each data set the number of all possible query candidates that comply with FactChecker's query model.\footnote{Three Wikipedia articles reference a total of six data sets.} These numbers demonstrate the difficulty of identifying the matching SQL query for each claim. For instance, Developer Survey Results 2017~\cite{Stackoverflow17}, whose data set consists of 154 columns, has more than one trillion query candidates.

\textbf{Number of Claims per Type.}
We found a total of 256 claims which could be verified by our system (i.e., numerical aggregates on relational data) from 37 text documents including Wikipedia articles. On the other hand, MARGOT identified 183 claims that are part of argument structures (i.e., argumentative claims) from the same set of articles. Note that these two set of claims are mostly exclusive with only one claim overlapping. Thus, the type of claims FactChecker is mainly interested about is very common even when compared against argumentative claims.

\section{Performance Tuning}
Here, we provide more experimental results on performance tuning.

\textbf{Effect of Parameter $\mathbf{p_T}$.}
Figure~\ref{pTFig} presents different verification trade-offs with respect to parameter $p_T$. Users can control this parameter depending on what they prefer between recall and precision. To effectively measure the influence of $p_T$, we need to ensure that the probabilities of query candidates directly affect the decision on whether a claim is correct or not. Thus, we verify each claim based on the evaluation of a query candidate with the highest probability, instead of verifying a claim by the existence of a query candidate that evaluates to the claimed value.

\textbf{Running Time per Data Set.}
Figure~\ref{comparisonByArticleFig} shows run times of different processing strategies, broken down by test case. This gives a better sense for the robustness of relative performance differences. Clearly, using all optimizations described in the previous sections yields best performance in the majority of cases.
